# Supplementary material for: Personalized Federated Learning via Amortized Bayesian Meta-Learning
Source: arXiv:2307.02222 source file (2023-07-05)
Supplement: Supplementary file 1 [file appendix.tex]

\newpage

\begin{appendices}
\crefalias{section}{appendix}
\crefalias{subsection}{appendix}
% \crefalias{subsubsection}{appendix}
The appendices are structured as follows. In Appendix \ref{app:framework}, we provide the proof procedure of Theorem \ref{stablitybeta}. The details of proof for Lemma \ref{contrative} is sketched in In Appendix \ref{appendix:ProofLemmas}. In Appendix \ref{app:add_exp}, we provide additional experiments and detailed setups.

\begin{spacing}{1.05}
 \listofappendices
\end{spacing}
\clearpage

\section{Elbo Derivation for General Framework} \label{app:framework}
\subsection{Detail of Derivation}
\begin{align*}
    &\log \Big[\prod_{i=1}^{M} p(\mathcal{D}_{i})\Big]=\log \Big[\int p(\theta)\big[\prod_{i=1}^{M} \int p(\mathcal{D}_{i} | \phi_{i}) p(\phi_{i} | \theta) d \phi_{i}\big] d \theta\Big] \\
    &\geq \int {q(\theta ; \psi)}\log \Big[\prod_{i=1}^{M} \int p(\mathcal{D}_{i} | \phi_{i}) p(\phi_{i} | \theta ) d \phi_{i}\Big] d \theta -\int {q(\theta ; \psi)} \frac{{q(\theta ; \psi)}}{p(\theta)} d \theta \\
    &= \mathbb{E}_{q(\theta ; \psi)}\Big[\log \big(\prod_{i=1}^{M} \int p(\mathcal{D}_{i} | \phi_{i}) p(\phi_{i} | \theta) d \phi_{i}\big)\Big]-\mathrm{KL}\big(q(\theta ; \psi) \| p(\theta)\big) \\
    &=\mathbb{E}_{q(\theta ; \psi)}\Big[\sum_{i=1}^{M} \log \big(\int p(\mathcal{D}_{i} | \phi_{i}) p(\phi_{i} | \theta) d \phi_{i}\big)\Big]-\mathrm{KL}\big(q(\theta ; \psi) \| p(\theta)\big) \\
    &\geq \mathbb{E}_{q(\theta ; \psi)}\Big[\sum_{i=1}^{M} \mathbb{E}_{q(\phi_{i} ; \lambda_{i})}\big[\log p(\mathcal{D}_{i} | \phi_{i})\big]-\mathrm{KL}\big(q(\phi_{i} ; \lambda_{i}) \| p(\phi_{i} | \theta)\big)\Big]-\mathrm{KL}\big(q(\theta ; \psi) \| p(\theta)\big) \\
    &=\mathcal{L}\big(\psi, \lambda_{1}, \ldots, \lambda_{M}\big) .
\end{align*}

\begin{align}
    \underset{\theta}{\arg \min } \Big[\sum_{i=1}^{M}-\mathbb{E}_{q_{\theta}(\phi_{i} | \mathcal{D}_{i})}\big[\log p(\mathcal{D}_{i} | \phi_{i})\big]+\operatorname{KL}\big(q_{\theta}(\phi_{i} | \mathcal{D}_{i}) \| p\left(\phi_{i} | \theta\right)\big)\Big]+\operatorname{KL}\big(q(\theta) \| p(\theta)\big).
\end{align}

\subsection{Comparison to existing Personlization FL approaches.}
A Compromise between Standard and Personalised FL. Interestingly, we show here that the FedPop framework allows existing FL approaches to be retrieved in certain regimes.
To this end, we assume that the prior 

\begin{align}
\text{pFedME:\quad} &\min_{w}\Big\{ F(w)=\frac{1}{N}\sum_{i=1}^{N} F_i(w) \Big\}, \text{where} \ F_i(w)=\min_{\theta}   \Big\{ f_i(\theta_i) + \frac{\lambda}{2} {\| \theta_i-w \|}^2 \Big\}, \end{align}

On the other hand, when
\begin{align}
\text{Per-FedAvg: \quad} &\min_{w}\Big\{ F(w)=\frac{1}{N}\sum_{i=1}^{N} F_i(\theta_i(w)) \Big\}, \text{where} \ \theta_i(w)=w-\alpha\nabla f_i(w).
\end{align}

This shows that FedPop stands for a subtle compromise between standard and personalised FL which should benefit clients with small data sets by pooling information via a common prior. Finally, in the extreme scenario where  is the null vector, our approach amounts to the Bayesian FL approach

\paragraph{Per-FedAvg: } In the simplest case where the prior is also assumed to be a Dirac delta function: $p(\w_{i} | \theta)=\delta(\mathrm{w}_{i}-\theta)$, and gradient descent is used, the local mode can be determined as:
$$
\w_{i}^{\mathrm{MAP}}=\theta-\alpha \nabla_{\w_{i}}\big[-\ln p(\mathcal{D}_{i} | \w_{i})\big]
$$

A simple way is to approximate $p(\w_i | \D_i, \theta)$ by a Dirac delta function at its local mode:
$$
p(\w_i | \D_i, \theta)=\delta\big(\w_i-\w_i^{\mathrm{MAP}}\big),
$$
where the local mode $\w_i^{\mathrm{MAP}}$ can be obtained by using maximum a posterior (MAP):
$$
\w_i^{\mathrm{MAP}}=\arg \max _{\w_i} \ln p\big(\D_i | \w_i\big)+\ln p(\w_i | \theta) .
$$
In the simplest case where the prior is also assumed to be a Dirac delta function: $p(\w_i | \theta)=\delta\big(\mathrm{w}_i-\theta\big)$, and gradient descent is used, the local mode can be determined as:
$$
\w_i^{\mathrm{MAP}}=\theta-\alpha \nabla_{\w_i}\big[-\ln p(\D_i | \w_i)\big],
$$
where $\alpha$ is the learning rate, and the truncated gradient descent consists of a single step of (6) (the extension to a larger number of steps is trivial). Given the point estimate assumption in (4), the upper-bound of the negative log-likelihood in (3) can be simplified to:
$$
\mathcal{L}^{(v)}(\theta)=\frac{1}{T} \sum_{i=1}^T-\ln p(\D_i | \w_i^{\mathrm{MAP}}) .
$$
Minimising the upper-bound of the negative loglikelihood in (7) w.r.t. $\theta$ represents the MAML algorithm [19]. This derivation also explains the intuition behind MAML, which finds a good initialisation of model parameters as illustrated in Figure $1 \mathrm{~b}$.

\paragraph{pFedME:}
\begin{align}
&\int p\left(\mathbf{X}_{j} | \w_{j}\right) p\left(\w_{j} | \boldsymbol{\theta}\right) \mathrm{d} \w_{j} \approx p\left(\mathbf{X}_{j} | \w_{j}^{*}\right) p\left(\w_{j}^{*} | \boldsymbol{\theta}\right) \operatorname{det}\left(\mathbf{H}_{j} / 2 \pi\right)^{-\frac{1}{2}} \\
-\log p(\mathbf{X} | \boldsymbol{\theta}) &\approx \sum_{j}\left[-\log p\left(\mathbf{X}_{j} | \hat{\w}_{j}\right)-\log p\left(\hat{\w}_{j} | \boldsymbol{\theta}\right)+\frac{1}{2} \log \operatorname{det}\left(\mathbf{H}_{j}\right)\right]\\
\text{when} \ p(\w | \mathbf{X},& \mathbf{y}, \boldsymbol{\theta}) \propto \mathcal{N}(\mathbf{y} ; \mathbf{X} \w, \mathbb{I}) \mathcal{N}(\w ; \boldsymbol{\theta}, \mathbf{Q})
\end{align}

\begin{align}
\text{VAMPIRE:\quad} &\min_{\theta} \Big\{\frac{1}{M} \sum_{i=1}^{M} \ln \mathbb{E}_{{q(\w_{i}; \lambda_i)}}\big[-p(\mathcal{D}_{i} | \w_{i})\big]\Big\}, \\
\text{where \quad}& \min _{\lambda_{i}} \mathcal{L}_{i}(\lambda_{i}, \theta)=\mathrm{KL}\big[q(\w_{i} ; \lambda_{i}) \| p(\w_{i} | \theta)\big]+\mathbb{E}_{q(\w_{i} ; \lambda_{i})}\Big[-\ln p(\mathcal{D}_{i} | \w_{i})\Big] .
\end{align}

\subsection{Correspondence between single step EM and gradient ascent}
With the addition of the auxiliary variables $\w_{i}$ we have that the overall objective for the server becomes
$$
\underset{\theta}{\arg \min } \frac{1}{N} \sum_{i=1}^{N} -\log \int p\left(\mathcal{D}_{i} | \w_{i}\right) p(\w_{i} | \theta) \mathrm{d} \w_{i} .
$$
By performing EM with a single gradient step for $\theta$ in the M-step (instead of full maximization), we are essentially doing gradient ascent on the original objective at 27 . To see this, we can take the gradient of Eq. 27 w.r.t. w where $Z_{i}=\int p(\mathcal{D}_{i} | \w_{i}) p(\w_{i} | \theta) \mathrm{d} \w_{i}$
$$
\begin{aligned}
&\frac{1}{N} \sum_{i} \frac{1}{Z_{i}} \int p\left(\mathcal{D}_{i} | \w_{i}\right) \frac{\partial p(\w_{i} | \theta)}{\partial \theta} \mathrm{d} \w_{i} \\
=&\frac{1}{N} \sum_{i} \int \frac{p(\mathcal{D}_{i} | \w_{i}) p(\w_{i} | \theta)}{Z_{i}} \frac{\partial \log p(\w_{i} | \theta)}{\partial \theta} \mathrm{d} \w_{i} \\
=&\frac{1}{N} \sum_{i} \int p(\w_{i} | \mathcal{D}_{i}, \theta) \frac{\partial \log p(\w_{i} | \theta)}{\partial \theta} \mathrm{d} \w_{i}
\end{aligned}
$$
where to compute Eq. 30 we see that we first have to obtain the posterior distribution of the local variables $\w_{i}$ and then estimate the gradient for $\theta$ by marginalizing over this posterior.

\newpage

\section{Additional Experiments and Setup Details} \label{app:add_exp}
\subsection{Setup Details}

\paragraph{aggregation}
For numerical stability, we parameterise the standard deviation point-wisely as $\sigma=\exp (\rho)$ when performing gradient update for the standard deviations of model parameters. The meta-parameters $\theta=\left(\boldsymbol{\mu}_\theta, \exp \left(\boldsymbol{\rho}_\theta\right)\right)$ are the initial mean and standard deviation of neural network weights, and the variational parameters $\lambda_i=\left(\boldsymbol{\mu}_{\lambda_i}, \exp \left(\boldsymbol{\rho}_{\lambda_i}\right)\right)$ are the optimised mean and standard deviation of those network weights adapted to task $\mathcal{T}_i$.

We also implement the re-parameterisation trick [34] when sampling the network weights from the approximated posterior to compute the expectation of the data log-likelihood in:
$$
\w_i=\boldsymbol{\mu}_{\lambda_i}+\epsilon \odot \exp \left(\boldsymbol{\rho}_{\lambda_i}\right)
$$
where $\epsilon \sim \mathcal{N}\left(0, \mathbf{I}_d\right)$, and $\odot$ is the element-wise multiplication. Given this direct dependency, the gradients of the cost function $\mathcal{L}_i^{(t)}$ in (9) with respect to $\lambda_i$ can be derived as:
$$
\left\{\begin{aligned}
\nabla_{\mu_{\lambda_i}} \mathcal{L}_i^{(t)} & =\frac{\partial \mathcal{L}_i^{(t)}}{\partial \w_i}+\frac{\partial \mathcal{L}_i^{(t)}}{\partial \boldsymbol{\mu}_{\lambda_i}} \\
\nabla_{\rho_{\lambda_i}} \mathcal{L}_i^{(t)} & =\frac{\partial \mathcal{L}_i^{(t)}}{\partial \w_i} \epsilon \odot \exp \left(\boldsymbol{\rho}_{\lambda_i}\right)+\frac{\partial \mathcal{L}_i^{(t)}}{\partial \boldsymbol{\rho}_{\lambda_i}}
\end{aligned}\right.
$$
After obtaining the variational parameters $\lambda_i$ in (10), we can apply Monte Carlo approximation by sampling $L_v$ sets of model parameters from the approximated posterior

\begin{align}
\text{oracle:}\quad \mu_S &= \sum_n^N \pi_n \mu_n, \quad \rho_s =\sum_{n=1}^N \pi_n\rho_n
\nonumber\\
\text{mean:}\quad \mu_S &= \sum_n^N \pi_n \mu_n, \quad \sigma^2_s =\sum_{n=1}^N \pi_n\sigma^2_n
=\sum_{n=1}^N \pi_n \big(\exp{\rho_n}\big)^2
\nonumber\\
\text{mixture:}\quad \mu_s &= \sum_n^N \pi_n \mu_n, \quad \sigma^2_s =\sum_{n=1}^N \pi_n\big(\sigma^2_n+\mu_n \mu_n^{\top}-\mu_S \mu_S^{\top}\big) 
\nonumber\\
\text{product:}\quad \mu_s &= \sigma_s^2\big(\sum_{n=1}^N \pi_n \sigma_n^{-2} \mu_n\big), \quad \sigma_s^{-2}=\sum_{n=1}^N \pi_n \sigma_n^{-2} \nonumber
\end{align}

$$
\begin{aligned}
& \mathcal{D}\left[\mathcal{N}\left(\mu_0, \Sigma_0\right) \| \mathcal{N}\left(\mu_1, \Sigma_1\right)\right]= \\
& \quad \frac{1}{2}\left(\operatorname{tr}\left(\Sigma_1^{-1} \Sigma_0\right)+\left(\mu_1-\mu_0\right)^{\top} \Sigma_1^{-1}\left(\mu_1-\mu_0\right)-k+\log \left(\frac{\operatorname{det} \Sigma_1}{\operatorname{det} \Sigma_0}\right)\right){ }_{(6}
\end{aligned}
$$
where $k$ is the dimensionality of the distribution. In our case, this simplifies to:
$$
\begin{aligned}
& \mathcal{D}[\mathcal{N}(\mu(X), \Sigma(X)) \| \mathcal{N}(0, I)]= \\
& \frac{1}{2}\left(\operatorname{tr}(\Sigma(X))+(\mu(X))^{\top}(\mu(X))-k-\log \operatorname{det}(\Sigma(X))\right) .
\end{aligned}
$$

\clearpage % don't remove
\end{appendices}
